# Supplementary material for: Maximizing Coverage Centrality via Network Design: Extended Version
Source: arXiv:1702.04082 source file (2017-10-09)
Supplement: Supplementary file 1 [file 7_1_appendix.tex]

\section*{Appendix}

\subsection*{Towards More General Settings}
\label{sec:general_settings}

The Coverage Centrality optimization problem on \textit{directed} graphs (e.g. our motivating example in Figure \ref{fig:motivation}) has the following setting: edges are added from or towards the target nodes $X$%\todo{here} %. We assume that the candidate sets of edges, $\Gamma$ includes the edges which have direction towards the target nodes. 
  ---i.e. directed edges in $\Gamma$ are of the form $(u,v)$ or $(v,u)$ where $u \in V\setminus X, v\in X$. %The direction is from $u$ to $v$. %\todo{does not match with pervious}
 
\begin{problem}\textbf{Coverage Centrality Optimization in Directed Graphs (CCO-D):} Given a directed network $G=(V,E)$, a target set of nodes $X \subset V$, a candidate set of edges $\Gamma$, and a budget $k$, find a set of edges $E_s\subset \Gamma$, such that $|E_s|\leq k$ and $C_m(X)$ is maximized.
\label{def:CCO-D}
\end{problem}

We assume the same constraint $S^2$ (as in the undirected graphs) on CCO-D. The next theorem shows that it is NP-hard to approximate within a factor greater than $(1- \frac{1}{e})$ even under this constraint.% and thus the same greedy algorithm described in Section~\ref{sec:greedy} can be applied with approximation guarantees.

\begin{thm}\label{thm:directed_approx_lower} CCO-D  under $S^2$ cannot be approximated within a factor greater than $(1- \frac{1}{e})$.
\end{thm}

The proof is in the extended version \cite{medya2017centrality}. The next theorem shows that the objective function in Problem~\ref{def:CCO-D} under $S^B$ is also monotone and submodular (same as in the undirected setting).% and thus the same greedy algorithm described in Section~\ref{sec:greedy} can be applied with approximation guarantees.

\begin{thm}\label{thm:submodular_wt} Given $X$, the objective function, $f(E_s)=C_m(X)$ in CCO-D is monotone and submodular.
\end{thm}

The proof for Theorem~\ref{thm:submodular_wt} is similar to that for Theorem~\ref{thm:submodular}. Based on this Theorem, our algorithm (BUS) can be applied to solve CCO-D with similar guarantees. In other words, our approach is agnostic to the direction of edges. Interestingly, Theorem \ref{thm:directed_approx_lower} and Theorem \ref{thm:submodular_wt} certifiy that GES achieves the best approximation for the constrained CCO-D problem.

We also briefly describe the CCO problem under different settings. In particular, we focus on possible restrictions on the set of candidate edges $\Gamma$. \textit{For undirected graphs}, \textbf{$S^1$:} $\Gamma$ is a subset of the set of all absent edges, \textbf{$S^2$:} $\Gamma$ consists of absent edges of the form $(u,v)$ where either $u$ or $v$ belongs to the target set $X$. For \textit{directed graphs}, \textbf{$S^4$:} $\Gamma$ is a subset of the set of all absent edges with arbitrary direction, \textbf{$S^5$:} $\Gamma$ consists of absent edges of the form $(u,v)$ where either $u$ or $v$ belongs to $X$,  with any direction.
  The hardness of these problems can be assessed with variations of the reasoning applied in Theorem $\ref{thm:nphard}$. Table \ref{table:problems} summarizes the different problem settings. We have already proven that the objective function is submodular under $S^2$ and $S^B$ (undirected) and under $S^5$ and $S^B$ (directed). Additionally, we prove that the objective functions for $S^2$ and $S^5$ are not submodular (see the extended version \cite{medya2017centrality}).% and thus all claims in Table \ref{table:problems} are proved.

 \begin{table}[ht]
\centering
%\vspace{-2mm}
\small
\begin{tabular}{| c | c | c| c| c| c| c|}
\hline
& \multicolumn{3}{c|}{\textbf{Undirected}} & \multicolumn{3}{c|}{\textbf{Directed}}\\
\hline
\textbf{Settings}& $S^1$ & $S^2$ & $S^2$, $S^B$ & $S^4$ & $S^5$ & $S^5$,$S^B$\\
\hline
\textbf{Submodular}& No & No & Yes & No & No & Yes \\
\hline
\end{tabular}
%\vspace{-2mm}
\caption{Summary of CCO problem under different settings. \label{table:problems}}
\vspace{-3mm}
 \end{table}

%\textbf{Discussion about $S2$ and $S3$: } We have argued that $S2$ is more realistic than $S1$. Though we provide the motivation about choosing $S2$ and $S3$ in Sec. \ref{sec:problem_definition}, we discuss it further here. Note that, our algorithms GES and BUS, are based on uncovered pairs. However, the graph is changing after the edge addition and the already covered paths might change and might not respect the constraint $S3$, but it does not affect our algorithms or our theoretical results because of the following: let $(u,v)$ is covered by our algorithm at a particular step. Now, shortest path between $(u,v)$ might change as graph is changing due to edge addition. But it will be covered as the paths can only change via the edges whose one of the end points is in $X$. 

\iffalse
\textbf{Non optimal behaviour of Greedy}

%Example of Greedy's non optimal behaviour
The submodularity property of the objective function ensures that Greedy algorithm produces a constant time approximation.

\begin{figure}[b]
    \centering
    \subfloat[Optimal]{\includegraphics[width=0.25\textwidth]{Figures/Greedy_O_NO/Greedy_nonoptimal.pdf}\label{fig:greedy_o}}
    \subfloat[Non Optimal Greedy]{\includegraphics[width=0.25\textwidth]{Figures/Greedy_O_NO/optimal.pdf}\label{fig:greedy_no}}
    \caption{Illustration of Greedy's non-optimal behaviour \label{fig:baselines_small_large}}
\end{figure}

\fi
